# Supplementary material for: High Performance Computing and Computational Intelligence Applications with MultiChaos Perspective
Source: arXiv:2212.00725 source file (2022-11-25)
Supplement: Supplementary file 1 [file appendix01.tex]

\begin{frontmatter}
\chapter{Appendix title}%\label{chap:appa}
\end{frontmatter}

%\section{}\label{}
