# Supplementary material for: High Performance Computing and Computational Intelligence Applications with MultiChaos Perspective
Source: arXiv:2212.00725 source file (2022-11-25)
Supplement: Supplementary file 2 [file appendix02.tex]

\begin{frontmatter}
\chapter{Appendix title}%\label{chap:appb}
\end{frontmatter}
